# Supplementary material for: DiffInfinite: Large Mask-Image Synthesis via Parallel Random Patch Diffusion in Histopathology
Source: arXiv:2306.13384 source file (2023-10-25)
Supplement: Supplementary file 1 [file framework.tex]

In this section we present \textit{Marcos cool method (MCM)} to sample from a distribution of a large image, by deploying a superposition of multiple realisations of the reverse time model learned during training on patches of smaller size. Even though we trained with discrete time steps, we formulate MCM in the general setting of a reverse time model in continuous time of \cite{song2021scorebased}. This is justified, since ancestral sampling used in DDPM is one particular discretization scheme of the reverse time model to the Variance Preserving SDE (VP SDE) in \cite{song2021scorebased}. The exploration of MCM for training in continuous time and differing underlying forward dynamics is dedicated to future research.

\subsection{The method}
Let $X\sim\mathcal{D}$ be the large image generating random variable taking values in $\mathbb{R}^{KD}$. Using the approach of latent diffusion models \adref{}, we first map to the latent space $\Phi(X)=Z \sim \mathcal{D}_{\Phi}$ taking values in $\mathbb{R}^{D}$, where we assume for simplicity the existence of an ideal encoder-decoder pair $(\Phi,\Psi)$ such that $\Psi(\Phi(X))=X$ is the identity on $\mathbb{R}^{KD}$. Common practice in histopathology is to tile a large image $X$ in small patches to perform a downstream task on the small patches \adref{}. The result of the downstream task is than again aggregated to some quantity on the large image. We intentionally omit the nomenclature of a whole slide image here, since with our computational resources it is not possible to generate an image of $100k \times 100k$ pixels. We still hope that the proposed sampling method MCM is a step further towards the generation of whole slide images. In the approach of \cite{zhang2023diffcollage} to generate large image content, a large image $u = [x^{(1)},...,x^{(m)}]$ is generated based on the assumption of conditional independence 
\begin{equation}
    q(x^{(i)}|x^{(i-1)},x^{(i-2)}) = q(x^{(i)}|x^{(i-1)}).
\end{equation}
The authors of \cite{zhang2023diffcollage} point out that the assumption of conditional independence  is not well-suited in cases of data distribution with long range dependence. For image generation in the medical context, we aim to permit long range dependence as we do not want to claim that the density of a given region depends only on one neighboring region. The key assumption of MCM is that the distribution of $k\times k$ cropped connected pixels is invariant wrt. to the cropped region in the latent image. To formulate this precisely we define the crop operation $\odot_{sub}$ that maps a flattened vector $c\in\{0,1\}^{d}$ representing a crop of $k\times k$ connected pixel and vector $v\in\mathbb{R}^{d}$ such that in $c \odot_{sub} v\in\mathbb{R}^{k^{2}}$ only the elements of $v_{i}$ are considered, where $c_{i}=0$.
The key assumption is 

\begin{assumption}
\label{ass:key}
For two arbitrary flattened crops $c_{1},c_{2}\in\{0,1\}^{D}$ of $k\times k$ connected pixels of a latent image $Z$ we have 
$c_{2}\odot_{sub} Z \stackrel{d}{=} c_{1}\odot_{sub} Z \sim \mathcal{C}_{\Phi}$, where $\mathcal{C}_{\Phi}$ is a distribution over $\mathbb{R}^{k^{2}}$.
\end{assumption}

The above assumption states that the distribution of a cropped latent image is invariant wrt. the location of the crop. \todo{comment on relation to wsi, maybe true in the inner of the wsi, but not the boundary not. For photographs this should be true, since it is assumed that the distirbution of the image is invariant wrt. the location of the camera. } 
To abbreviate notation we define the random variable $Y= C \odot_{sub} Z$ with $Y\sim\mathcal{C}_{\Phi}$, where $C$ is a uniform random variable over all possible crops of $k\times k$ connected latent pixels. For a given crop $c$, we define our latent diffusion forward process by simply placing a diffusive process only on the $k\times k$ cropped pixels such that the pixelwise forward dynamics in latent space are given by
\begin{equation}
\label{eq:forward}
    dy^{c}_{t} =
    \mu(t)y^{c}_{t}dt + \sigma(t)dW_{t}, \quad y^{c}_{0} = c \odot_{sub} Z
\end{equation}
By \Cref{ass:key} we have $y^{c_{1}}_{t}\stackrel{d}{=}y^{c_{2}}_{t}$ for any time point $t\in[0,T]$ and any two crops $c_{1},c_{2}$ such that $y^{c_{1}}_{t}$ and $y^{c_{2}}_{t}$ share the same score function. Hence, following \cite{anderson1982} we find for any $c$ the reverse time model $\bar{y}^{c}_{t}=y^{c}_{T-t}$ to \cref{eq:forward} with dynamics
\begin{equation}
\label{eq:reverse}
    d\bar{y}^{c}_{t} =
    \bar{\mu}(t)\bar{y}^{c}_{t}dt - \bar{\sigma}^{2}(t)\nabla_{y}\log(p(y^{c}_{t},T-t))dt + \bar{\sigma}(t)d\bar{W}_{t}
\end{equation}
with $\bar{\mu}(t)=\mu(T-t), \bar{\sigma}(t)=\sigma(T-t)$ and $\bar{W}_{t}=W_{T-t}$,
where the density $p(\cdot,t)$ at time $t$ does not depend on the crop $c$. 
To sample a whole latent image of size $lk^{2}$, we could deploy the reverse time model $l$ times and stack the samples together after sampling. This would lead to a latent image with regions of low correlation, since $\nabla_{y}p(y,t)$ is not able to take into account the realisations of neighboring regions. 
Towards the goal of a sampling method with long range dependence we propose MCM. Let $SM$ be any a recursive sampling method of the reverse time model in \Cref{eq:reverse} over the discretized time steps $0=t_{1}<...<t_{N}=T$ with recursive scheme
\begin{equation}
\label{eq:sm_step}
    y^{c}_{t_{n-1}} = SM(y^{c}_{t_{n}}).
\end{equation}
We first sample $Z_{T}\sim\mathcal{N}(0,I_{D})$ with dimension $D$ according to the full latent space. Given $Z_{t_{n}}$ we first sample $c^{n}_{1},...,c^{n}_{m}$ flattened overlapping, but non equal crops that cover all latent pixels. Secondly, we calculate $y^{c^{n}_{k}}_{t_{n}}=c^{n}_{k}\odot_{sub}Z_{t_{n}}$ for all $k\in\{1,...,m\}$ and perform one step of SM according to \Cref{eq:sm_step} resulting in $y^{c^{n}_{1}}_{t_{n-1}}, y^{c^{n}_{2}}_{t_{n-1}},....,y^{c^{n}_{m}}_{t_{n-1}}$. Since $c^{n}_{1},...,c^{n}_{m}$ are overlapping, we have multiple values for some pixels. Let $s_{l\to c}$ be the map that maps a pixel $i\in\{1,...,D\}$ of the latent space to the crop of it's first appearance in $c^{n}_{1},...,c^{n}_{m}$. For $i\in\{1,...,D\}$ let $k_{i}$ be the pixel in the crop $s_{l\to c}(i)$ that corresponds to $i$ in the latent space. Using $s_{l\to c}$ and $k_{i}$, we define
\begin{equation}
    Z_{t_{n-1},i} = SM(y^{s_{l\to c}(i)}_{t_{n}})_{k_{i}}.
\end{equation}
Doing so for all $i\in\{1,...,D\}$, we recursively define $Z_{t_{n-1},i}$, given $Z_{t_{n-1}}$ and the crops $c^{n}_{1},...,c^{n}_{m}$. Therefore, we define the density of $Z_{t_{n-1}}$ by
\begin{equation}
    Z_{t_{n-1}} \sim p_{SM_{n}}(z|Z_{t_{n}},c^{n}_{1},...,c^{n}_{m})
\end{equation}
Since $Z_{T}$ and $c^{N}_{1},...,c^{N}_{m}$ are independent, using Bayes theorem leads to
\begin{align}
    p_{SM_{N}}(z|Z_{T},c^{N}_{1},...,c^{N}_{m}) &= \frac{p_{SM_{N}}(z,Z_{T},c^{N}_{1},...,c^{N}_{m})}{p_{SM_{N}}(Z_{T},c^{N}_{1},...,c^{N}_{m})} 
    = \frac{p_{SM_{N}}(z,Z_{T})p_{SM_{N}}(c^{N}_{1},...,c^{N}_{m})}{p_{SM_{N}}(Z_{T})p_{SM_{N}}(c^{N}_{1},...,c^{N}_{m})} \\
    &= \frac{p_{SM_{N}}(z,Z_{T})}{p_{SM_{N}}(Z_{T})} = p_{SM_{N}}(z|Z_{T})
\end{align}
Repeating the argument for all steps $1\leq n \leq N$ leads to 
\begin{equation}
    Z_{0} \sim p_{SM_{1}}(z|Z_{t_{1}},...,Z_{t_{N}}) 
\end{equation}
and finally, if $SM$ induces a discrete Markov chain
\begin{equation}
    Z_{t_{n-1}} \sim p_{SM_{n}}(z|Z_{t_{n}}).
\end{equation}
For now we assume $Z_{0} \sim p_{SM_{1}}(z|Z_{t_{1}},...,Z_{t_{N}})$. Let $(z_{t})_{t\in[0,T]}$ be the forward process of a diffusion model on the full latent space with dynamics
\begin{equation}
    dz_{t} = \mu(t)z_{t}dt + \sigma(t)dW_{t},\quad z_{0}=Z
\end{equation}
with reverse time model
\begin{equation}
    d\bar{z}_{t} = \bar{\mu}(t)\bar{z}_{t}dt - \bar{g}(t)\nabla_{z}\log(p_{z}(\bar{z_{t}},T-t))dt + \bar{g}(t)d\bar{W}_{t},
\end{equation}
discretization scheme
\begin{equation}
    z_{t_{n-1}} = SM(z_{t_{n}})
\end{equation}
and resulting distribution $z_{0} \sim \hat{D}_{\Phi,N}$ with density $\hat{p}_{\phi,N}$. We aim to show
\begin{equation}
\label{eq:conv_kldiv}
    D_{KL}(\hat{p}_{\phi,N}\Vert p_{SM_{1}}(z|Z_{t_{1}},...,Z_{t_{N}})) \leq e_{n}\to 0 \quad \textit{for}\,\,n\to \infty
\end{equation}
and that for the correlation function satisfies
\begin{equation}
    \rho(z_{0,i},z_{0,j}) > 0 \quad \textit{for all}\,\, i,j\in\{1,...,D\},
\end{equation}
such that any two pixels of the image have positive correlations. 
Assume that $SM$ is a well justified samlpling method we have
\begin{equation}
    D_{KL}(\hat{p}_{\phi,N}\Vert p_{\phi}) \leq e_{n}\to 0 \quad \textit{for}\,\,n\to \infty
\end{equation}
Hence, by triangle inequality
\begin{equation}
    D_{KL}( p_{SM_{1}}(z|Z_{t_{1}},...,Z_{t_{N}}) \Vert p_{\phi}) \leq e_{n}\to 0 \quad \textit{for}\,\,n\to \infty
\end{equation}
BUT, how to show \Cref{eq:conv_kldiv}?

\newpage
that is the density of the $(n-1)-th$ step under the sampling method SM.
we have multiple values for some pixels and we reconstruct $Z_{t_{n-1}}$ from $y^{c_{1}}_{t_{n-1}}, y^{c_{2}}_{t_{n-1}},....,y^{c_{m}}_{t_{n-1}}$ by first padding zero values to the missing entries of $y^{c_{k}}_{t_{n-1}}$ such that
\begin{equation}
    z^{c_{k}}_{t_{n-1}} = Pad(y^{c_{k}}_{t_{n-1}}) \in \mathbb{R}^{D}
\end{equation}
and second we define $Z_{t_{n-1}}=0_{D}$ and assign to every pixel $i$ the value of the first crop that considers $i$ such that
\begin{equation}
    Z_{t_{n-1},i} = z^{c_{k^{\star}}}_{t_{n-1},i},\quad\textit{with}\quad k^{\star} = \argmin_{\stackrel{k=1,...,m}{z^{c_{k}}_{t_{n-1}}\not=0}}\{z^{c_{1}}_{t_{n-1}},....,z^{c_{m}}_{t_{n-1}}\}.
\end{equation}

For pixel $i$ we fix an arbitrary crop $C$ with $C_{i}=1$. The reverse time model \Cref{eq:reverse} with $y_{t,j} = 0$, for $C_{j}=0$ can be used to sample a latent image $z^{i}$ covering pixel $i$.

Let $\bar{c}$ be the complement crop to $c$ such that $c + \bar{c}= 1_{D}$.
Ideally we would define a sampling method such that for any cropped latent image  we condition the cropped region $y^{c}_{0}$ on all of the non-cropped part of the image, such that
\begin{equation}
    Pad(y^{c}_{0}) + (1-c) \odot Z \sim \mathcal{D}_{\Phi}
\end{equation}
where Pad fills the cropped-out values with zeros and $\odot$ is elementwise multiplication. Hence, the distribution we aim for is
\begin{equation}
    y^{c}_{0} \sim p_{0}(y | (1-c)\odot Z) = \frac{p(y,(1-c)\odot Z)}{p((1-c)\odot Z)}
\end{equation}

Let $SM$ be a sampling method of the reverse time model in \Cref{eq:reverse} over the discretized time steps $0=t_{1}<...<t_{N}=T$ with recursive scheme
\begin{equation}
\label{eq:sm_step}
    y^{c}_{t_{n-1}} = SM(y^{c}_{t_{n}}).
\end{equation}
We first sample $Z_{T}\sim\mathcal{N}(0,I_{D})$ with dimension $D$ according to the full latent space. Given $Z_{t_{n}}$ we first sample $c_{1},...,c_{m}$ flattened overlapping, but non equal crops that cover all latent pixels. Secondly, we calculate $y^{c_{k}}_{t_{n}}=c_{k}\odot_{sub}Z_{t_{n}}$ for all $k\in\{1,...,m\}$ and perform one step of SM according to \Cref{eq:sm_step} resulting in $y^{c_{1}}_{t_{n-1}}, y^{c_{2}}_{t_{n-1}},....,y^{c_{m}}_{t_{n-1}}$. Since $c_{1},...,c_{m}$ are overlapping, we have multiple values for some pixels. Let $k\to c$ be the map that maps a pixel $i\in\{1,...,D\}$ of the latent space to the crop of it's first appearance in $c_{1},...,c_{m}$. Using $s$, we define
\begin{equation}
    Z_{t_{n-1},i} = SM(y^{s(i)}_{t_{n}}).
\end{equation}

$Z_{t_{n-1}}$ from $y^{c_{1}}_{t_{n-1}}, y^{c_{2}}_{t_{n-1}},....,y^{c_{m}}_{t_{n-1}}$ by first padding zero values to the missing entries of $y^{c_{k}}_{t_{n-1}}$ such that
\begin{equation}
    z^{c_{k}}_{t_{n-1}} = Pad(y^{c_{k}}_{t_{n-1}}) \in \mathbb{R}^{D}
\end{equation}
and second we define $Z_{t_{n-1}}=0_{D}$ and assign to every pixel $i$ the value of the first crop that considers $i$ such that
\begin{equation}
    Z_{t_{n-1},i} = z^{c_{k^{\star}}}_{t_{n-1},i},\quad\textit{with}\quad k^{\star} = \argmin_{\stackrel{k=1,...,m}{z^{c_{k}}_{t_{n-1}}\not=0}}\{z^{c_{1}}_{t_{n-1}},....,z^{c_{m}}_{t_{n-1}}\}.
\end{equation}

\newpage
If SM is Euler we have
\begin{equation}
    Z_{t_{n-1},i} = Z_{t_{n},i} + \mu(t_{n})Z_{t_{n},i}\Delta t - \bar{g}^{2}(t_{n})\nabla_{y}\log(p(y^{c_{k^{\star}}}_{t_{n}},t_{n}))\Delta t + g(t_{n})\Delta W_{n}
\end{equation}
with bayes theorem by independence of $z_{T}$ and $c^{T}_{1},...,c^{T}_{m}$
\begin{align}
    z_{t_{N-1}} \sim p(z_{t_{N-1}}|z_{T},c^{T}_{1},...,c^{T}_{m}) &= \frac{p(z_{t_{N-1}},z_{T},c^{T}_{1},...,c^{T}_{m})}{p(z_{T},c^{T}_{1},...,c^{T}_{m})} \\
    &= \frac{p(z_{t_{N-1}},z_{T})p(c^{T}_{1},...,c^{T}_{m})}{p(z_{T})p(c^{T}_{1},...,c^{T}_{m})} \\
    &= p(z_{t_{N-1}}|z_{T})
\end{align}
and similar
\begin{equation}
    z_{t_{N-2}} \sim p(z_{t_{N-2}}|z_{t_{N-1}},z_{T},c^{t_{N-1}}_{1},...,c^{t_{N-1}}_{m}) = p(z_{t_{N-2}}|z_{t_{N-1}},z_{T}).
\end{equation}
Repeating for every step
\begin{equation}
    z_{t_{n-1}} \sim p(z_{t_{n-1}}|z_{t_{n}},z_{t_{n+1}},...,z_{T},c^{t_{n}}_{1},...,c^{t_{n}}_{m}) = p(z_{n-1}|z_{t_{n}},...,z_{T})
\end{equation}
and finally
\begin{equation}
    z_{0} \sim p(z_{0}|z_{t_{1}},...,z_{T})
\end{equation}
So to what corresponds $p(z_{t_{n-1}}|z_{t_{n}})$? Assume the reverse time model
\begin{equation}
    d\bar{z}_{t} = \bar{\mu}(t)\bar{z}_{t}dt - \bar{\sigma}^{2}(t)\nabla_{z}\log(p_{z}(\bar{z}_{t},T-t))dt + \bar{\sigma}(t)d\bar{W}_{t}
\end{equation}
to the full latent forward diffusion process
\begin{equation}
\label{eq:forward}
    dz_{t} =
    \mu(t)z_{t}dt + \sigma(t)dW_{t}, \quad z_{0} = Z.
\end{equation}
Let $z^{\star}_{0}$ be the output of the full reverse model following
\begin{equation}
    z^{\star}_{0}\sim p_{z}(z^{\star}_{0}|z^{\star}_{t_{1}},...z^{\star}_{t_{N-1}},z_{N}).
\end{equation}
How is the relation of $z^{\star}_{0}$ and $z_{0}$. Try to write $p_{z}$ in terms of $p$.
\begin{equation}
    p(z) = p_{1} \otimes p_{2}\otimes ... \otimes p_{D}(z_{1},z_{2},...,z_{D}) 
\end{equation}
\newpage
Let $p_{k^{\star}}$ be the density of $z^{c_{k^{\star}}}_{t_{n-1},i}$ and  $p_{z}(z,t)$ the denisty of $(z_{t})_{t\in[0,T]}$ with dynamics 
\begin{equation}
    dz_{t} =
    \mu(t)z_{t}dt + \sigma(t)dW_{t}, \quad z_{0} = Z
\end{equation}
We aim to show that 
\begin{equation}
    p_{k^{\star}} = p_{z}(z,t).
\end{equation}
We calculate
\begin{equation}
...    
\end{equation}
where $p_{z}(z,t),$ is the density of
\begin{equation}
    \mathbb{E}_{c}\left[p(z_{t_{n-1},i}|z_{t_{n-1}})\right]=\frac{1}{K}\sum_{c=(c_{1},...,c_{m})}p(z_{t_{n-1},i}|z_{t_{n}},c_{1},...,c_{m})
\end{equation}
\begin{equation}
    p(z_{t_{n-1},i}|z_{t_{n-1}},c_{1},...,c_{m}) \not=\sum_{k=1}^{m} p(z_{t_{n-1},i}|z_{t_{n-1}},c_{k})
\end{equation}

\begin{equation}
    p_{z}(z_{t_{n-1}},t_{n-1}) = p_{i_{1}} \otimes p_{i_{2}} \otimes ... \otimes p_{i_{k^{2}}}
\end{equation}

\newpage
Repeating this procedure for every crop $C$ of size $k\times k$with $C_{i}=1$ leads to a superposition of generated images that all cover the pixel $i$ after a total of $k
^{2}$ realisations of the reverse time model and calculating $\frac{1}{k}\sum_{l=1}^{k}z_{i}|C$ leads to a sample with maximal long range correlation, given the dimension of the latent space diffusion. Doing so is not feasible, since this would require $d^{2}k^{2}$ realisations of the reverse time model for the generation of a single sample. Nevertheless, we aim to introduce a sampling method, where all $z_{i}|C$ are admissible to foster long range dependence.

Given $z_{t}$ we first sample a single pixel and second one possible path $(\tilde{z}_{t}|C)_{t\in[0,T]}$ such that $\tilde{z}_{t}=z_{t}$

approximate $\frac{1}{k}\sum_{l=1}^{k}z_{i}|C$ over different realisations of the reverse time model, by 

allowing all the samples $z_{i}|C$ to be ass

\newpage
\ck{:does this follow from the assumption?}. In the case of landscape generation, neglecting for example 
\begin{equation}
    q(x^{(i)}|x^{(i-1)},x^{(i-2)})=0 \quad \land \quad q(x^{(i)}|x^{(i-1)})>0
\end{equation}
might cause limited harm. \todo{find good example to illustrate that the above needs to be considered in the medical context, for example because cell type in region $x^{(i-1)}$ and in region $x^{(i-2)}$ can not be part of the same WSI}.
conditions the sampling on a fixed, already generated image assuming

large image in the latent space is invariant wrt. the cropped region. To be more precise, let 

\newpage

In \cite{zhang2023diffcollage} the reverse process
\begin{equation}
    du_{t} = -(1+\eta^{2})\sigma^{\prime}_{t}\sigma_{t}\nabla_{u}\log(q(u_{t})dt + \eta\sqrt{\sigma^{\prime}_{t}\sigma_{t}}dW_{t}
\end{equation}
is used to generate samples $u = [x^{(1)},...,x^{(m)}]$ from a high dimensional distribution $\mathcal{D}$ based on the assumption of conditional independence 
\begin{equation}
    q(x^{(i)}|x^{(i-1)},x^{(i-2)}) = q(x^{(i)}|x^{(i-1)}).
\end{equation}
The authors of \cite{zhang2023diffcollage} point out that the assumption of conditional independence  is not well-suited in cases of data distribution with long range dependence. For image generation in the medical context, we aim to permit long range dependence as we do not want to claim that the density of a given region depends only on one neighboring region \ck{:does this follow from the assumption?}. In the case of landscape generation, neglecting for example 
\begin{equation}
    q(x^{(i)}|x^{(i-1)},x^{(i-2)})=0 \quad \land \quad q(x^{(i)}|x^{(i-1)})>0
\end{equation}
might cause limited harm. \todo{find good example to illustrate that the above needs to be considered in the medical context, for example because cell type in region $x^{(i-1)}$ and in region $x^{(i-2)}$ can not be part of the same WSI}. 
Let $X$ be the large image generating random variable following the unknown distribution $\mathcal{D}$ with density $p$. To model a random and independent crop with known distribution $\mathcal{C}$ and density $p_{C}$, we define the random vector $C\sim\mathcal{C}$ that takes values only in $\{0,1\}^{d}$. The forward process of \textit{our very cool model} follows the dynamics
\begin{equation}
    du_{t} = C\left[\mu(t)u_{t}dt + \sigma(t)dW_{t}\right], \quad u_{0} = Cx_{0}
\end{equation}
with reverse time model \cite{songscore2020}, \cite{anderson1982}
\begin{equation}
    d\bar{u}_{t} = C\left[\bar{\mu}(t)\bar{u}_{t}dt - \bar{\sigma}^{2}(t)\nabla_{u}\log(q(\bar{u}_{t},t))dt + \bar{\sigma}(t)\bar{W}_{t}\right]
\end{equation}
where $\bar{u}_{t}=u_{T-t}$, $\bar{W}_{t}=W_{T-t}$, $\bar{\mu}(t) = \mu(T-t)$, $\bar{\sigma}(t)=\sigma(T-t)$ and $q(\cdot,t)$ is the density of $u_{t}$. To approximate the score function by $s_{\theta}$ we aim for
\begin{equation}
    \theta^{\star} = \argmin_{\theta}\mathbb{E}_{t}\left\{\lambda(t)\mathbb{E}_{t,u_{0}}\mathbb{E}_{u_{t}|u_{0}}\left[\left\Vert s_{\theta}(u_{t},t)-\nabla_{u_{t}}q_{0t}(u_{t}|u_{0})\right\Vert^{2}_{2}\right]\right\},
\end{equation}
where $q_{0t}(\cdot,t|u_{0})$ is the denisty of $u_{t}|u_{0}$.

Since $X$ and $C$ are independent, the joint of $(X,C)$ is $p(x,y)=p(x)p(c)$ such that
\begin{comment}
\begin{equation}
    p(x) = \int_{\{0,1\}^{d}\times\mathbb{R}^{d}}p(x,y)dy = p(x)\int_{\{0,1\}^{d}\times\mathbb{R}^{d}}p(y)dy 
\end{equation}
\end{comment}

\vspace{0.5cm}
\textbf{Approach 2 (Define just a new samplign method)}
 Towards the goal of circumnavigating the assumption of conditional independence we define for every dimension $i$ in the data domain the random variable $C_{d}$ that takes only values in $\{0,1\}$ to model the random crop of $K=\sum_{d=1}^{D}C_{d}$ connected pixels following a known distriburtion $C\sim\mathcal{C}$. Aiming to generate $X\sim\mathcal{D}$ we train a diffusion model of dimension $K$ with starting value $X_{0} = CX$ and forward proecess
 \begin{equation}
     dx_{t} = -\frac{1}{2}\beta(t)x_{t}dt + \sqrt{\beta(t)}dw_{t}
 \end{equation}
\begin{equation}
    dx_{t} = -(1+\eta^{2})\sigma^{\prime}_{t}\sigma_{t}\nabla_{u}\log(q(u_{t})dt + \eta\sqrt{\sigma^{\prime}_{t}\sigma_{t}}dW_{t}
\end{equation}
 
\vspace{0.5cm}
\textbf{Approach 1 (Define new model)}
Towards the goal of circumnavigating the assumption of conditional independence we define for every dimension $i$ in the data domain the piecewise constant process $C_{t, d}$ taking only values in $\{0,1\}$. To model the random crop of $K=\sum_{d=1}^{D}C_{t,d}$ connected pixels at time $t$, we assume in addition that all pixels with $C_{t_d}$ are connected, when $C_{t}$ is reshaped as an image. We define the forward dynamics of DiffInfinite by
\begin{equation}
    dX_{t} = \mu(t)C_{t}X_{t}dt +\sigma(t)C_{t}dW_{t},
\end{equation}
where the processes $C$ and $W$ are assumed to be independent. Justified by the latter assumption, we treat $C_{t}$ as a deterministic function. For a fixed realisation of $C$ and condition $y$ we follow Equation (48) of \cite{song2021scorebased} to derive the dynamics of the conditional reverse time model 
\begin{equation}
    d\bar{X}_{t} = \bar{\mu}(t)\bar{C}(t)\bar{X}_{t}dt -  \bar{C}(t)\bar{\sigma}(t)\nabla_{x}\log(p(\bar{X}_{t},T-t|y))dt + \bar{C}_{t}\bar{\sigma}(t)d\bar{W}_{t},
\end{equation}
where $\bar{X}_{t} = X_{T-t}$. With $Z_{t} = \exp\left(-\int^{t}_{0}\mu(s)C_{s}ds\right)$ we can reparameterizing the forward process to 
\begin{equation}
    X_{t} = Z_{t}\left(x_{0} + \int^{t}_{0}\frac{\sigma(s)C_{s}}{Z_{s}}dW_{s}\right) \sim\mathcal{N}(m_{t},\tau^{2}_{t})
\end{equation}
to show that $X_{t}$ is Gaussian for every $t\in[0,T]$. For positive $\mu$ we have $\int^{t}_{0}\mu(s)C_{s}ds\leq \int^{t}_{0}\mu(s)C_{s}ds$ and hence we find for the mean
\begin{equation}
   \vert m_{t} \vert = Z_{t}\vert x_{0} \vert  \to 0,\quad \textit{for} \,\, t \to \infty
\end{equation}
if $\mu(t)\to\infty$ for $t\to\infty$. For the variance observe
\begin{equation}
    \tau^{2}_{t} = \exp\left(-2\int^{t}_{0}\mu(s)C_{s}ds\right) \int^{t}_{0}\frac{\sigma^{2}(s)C^{2}_{s}}{Z^{2}_{s}}ds \geq \exp\left(-2\int^{t}_{0}\mu(s)ds\right) \int^{t}_{0}\frac{\sigma^{2}(s)}{Z^{2}_{s}}ds = \tilde{\tau}^{2}_{t}.
\end{equation}
Hence, the variance dominates the variance of the initial model with $C_{t}\equiv 1$. Since $X_{t}$ is Gaussian, the loss function reduces to
\begin{align}
    \Vert s_{\theta}(X_{t},t) - \log(p(X_{t},t))\Vert^{2} &= \Vert s_{\theta}(X_{t},t) +\frac{Z}{\tau}_{t}\Vert^{2} =\frac{1}{\tau_{t}}\Vert \tau_{t} s_{\theta}(X_{t},t) + Z\Vert^{2} \\
    &\leq \frac{1}{\tilde{\tau}^{2}_{t}}\Vert \tau_{t} s_{\theta}(X_{t},t) + Z\Vert
    = \Vert \frac{\tau_{t}}{\tilde{\tau}_{t}} s_{\theta}(X_{t},t) +\frac{Z}{\tilde{\tau}_{t}}\Vert.
\end{align}
Aiming for $\tilde{s}_{\theta}(X_{t},t) = \frac{\tilde{\tau}_{t}}{\tau_{t}}$ we can minimize the RHS to minimize the LHS.
$\Rightarrow$ loss does not change\newline
\todo{Biggest problem is that coefficient functions are no longer continuous, so time reversal result does not hold}
