# Supplementary material for: DiffInfinite: Large Mask-Image Synthesis via Parallel Random Patch Diffusion in Histopathology
Source: arXiv:2306.13384 source file (2023-10-25)
Supplement: Supplementary file 2 [file comp2diffcollage.tex]

\reviewerC{
To compare our method to DiffCollage we generate 200 images of size $2048 \times 2048$ using the method proposed in \cite{zhang2023diffcollage} and compute the metrics used in the main paper to evaluate DiffInfinite. According to \Cref{tab:comp2diffcollage} DiffInfinite scores higher in IP and IR, while DiffCollage has a higher authenticity score and a lower $\boldsymbol{C_{T}}$ score. The slight improvement of the authenticity score comes at the cost of a very low IR, indicating substantial differences in the distributions of the real and the generated samples. We conjecture that this is a result of the tiling artefacts observable in \Cref{fig:collagevsinfinite}.}

\begin{table}[!h]
    \centering
    \caption{Comparison of DiffCollage and DiffInfinite.}
    \begin{tabular}{llllll}
        \toprule
         & \textbf{IP} \textuparrow & \textbf{IR} \textuparrow & $\boldsymbol{A}$ \textuparrow & $\boldsymbol{C}_{T}$ $\downuparrows$\\
         \midrule
         DiffCollage & 0.88 & 0.08 &  \textbf{0.97} & \textbf{7.00} \\
         DiffInfinite & \textbf{0.98} & \textbf{0.44} &  0.95 & 10.96 \\
    \end{tabular}
    \label{tab:comp2diffcollage}
\end{table}
